# Supplementary material for: Characterization of methanol as a magnetic field tracer in star-forming regions
Source: arXiv:1802.05764 source file (2018-02-15)
Supplement: Supplementary file 1 [file supp_9.pdf]

# Supplementary: Characterization of methanol as a magnetic field tracer in star-forming regions


Boy Lankhaar and Wouter Vlemmings

*Department of Space, Earth and Environment,*
*Chalmers University of Technology,*
*Onsala Space Observatory, 439 92 Onsala, Sweden**

Gabriele Surcis

*Joint Institute for VLBI ERIC, Postbus 2,*
*7990 AA Dwingeloo, The Netherlands and*
*INAF, Osservatorio Astronomico di Cagliari Via della Scienza 5, I-09047 Selargius, Italy*

Huib Jan van Langevelde

*Joint Institute for VLBI ERIC, Postbus 2,*
*7990 AA Dwingeloo, The Netherlands and*
*Sterrewacht Leiden, Leiden University,*
*Postbus 9513, 2330 RA Leiden, the Netherlands*

Gerrit C. Groenenboom and Ad van der Avoird

*Theoretical Chemistry, Institute for Molecules and Materials,*
*Radboud University, Heyendaalseweg 135,*
*6525 AJ Nijmegen, The Netherlands*



(Dated: October 25, 2017)

* lankhaar@chalmers.se

## NON-LINEAR ZEEMAN EFFECTS

Figure 2 in the paper shows the non-linear Zeeman effects in methanol that prevail already at low magnetic fields. Here, we will discuss the origins of these non-linear effects and their consequences for the description of the Zeeman parameters of methanol.

The Zeeman shift of a maser line emitted in a magnetic field $B$ is defined as half the difference between the energies where the right- and left-circularly polarized radiation have their maximum intensities: $\Delta E(B) = [E_{\rm rcp}(B) - E_{\rm lcp}(B)]/2$, and the g-factor is

$$g(B) = -\frac{\Delta E(B)}{\mu_N B}, \tag{1}$$

where $\mu_N$ is the nuclear magneton. Usually the Zeeman shifts depend linearly on $B$ and the Landé g-factors are constant. Supplementary Figure 1 shows the g-factors of the different hyperfine components of the 6.7 GHz ($5_{15}\ A_2 \rightarrow 6_{06}\ A_1$) and 36 GHz ($4_{-1}\ E \rightarrow 3_0\ E$) methanol maser transitions over a magnetic field range from 0 to 60 mG. It is clear from this figure that for several hyperfine-state resolved transitions the g-factors are not constant. Especially for the 36 GHz transition in panel (b) of the figure, we observe a strong magnetic field dependence of the g-factors for two of the hyperfine lines: for one of them it varies by more than a factor of three. We also observe in this figure that there is a large variation among the g-values of different hyperfine transitions, with both positive and negative signs occurring.

These non-linear Zeeman shifts are caused by mixing of the hyperfine states. This happens in particular when the energy gap between hyperfine levels is of the same order of magnitude as their Zeeman shifts in the external magnetic field. The most striking case, which produces the strongest magnetic field dependence of the g-values in panel (b) of Supplementary Figure 1, is a mixing of the $F = 4$ and $F = 5$ levels of the $4_{-1}\ E$ state, which are only 0.34 kHz apart. Also in other cases the energy gaps between hyperfine levels are as small as about 2 kHz and there is substantial mixing of hyperfine levels with $\Delta F = 1$. It will be clear that $F$ is no longer a good quantum number in such cases.

Since particular hyperfine levels are mixed by the external magnetic field, the nature of the transition between such levels changes with the magnetic field as well. Supplementary Figure 2 illustrates the influence of the magnetic field on the Einstein A-coefficients of the 6.7 GHz ($5_{15}\ A_2 \rightarrow 6_{06}\ A_1$) and 36 GHz ($4_{-1}\ E \rightarrow 3_0\ E$) transitions. For all hyperfine

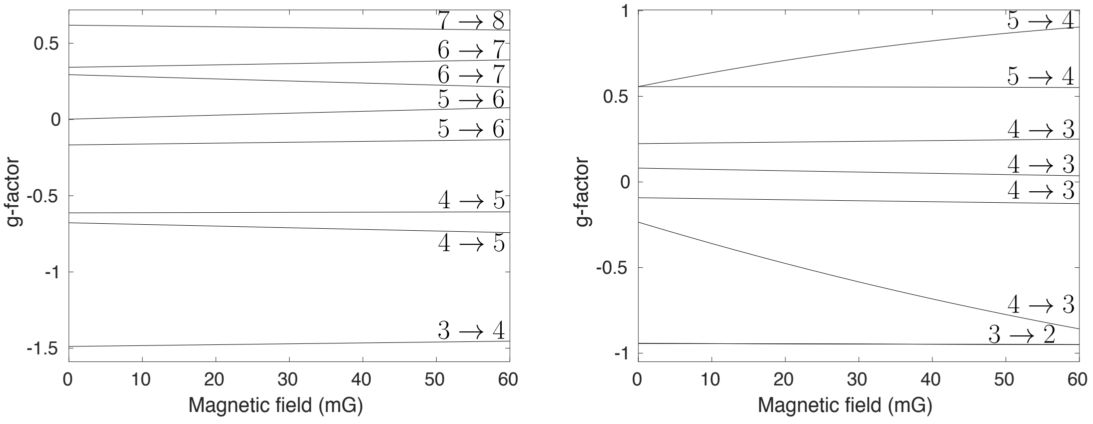


(a) (b)

Supplementary Figure 1: Magnetic field dependence of the g-factors of the strongest hyperfine transitions within the 6.7 GHz ($5_{15}\ A_2 \rightarrow 6_{06}\ A_1$) (a) and 36 GHz ($4_{-1}\ E \rightarrow 3_0\ E$) (b) methanol maser lines. The different components are labeled $F \rightarrow F'$ with their initial and final $F$ values, which are good quantum numbers for $B = 0$.

components of both torsion-rotation transitions, we observe a significant magnetic field dependence of the A-coefficients.

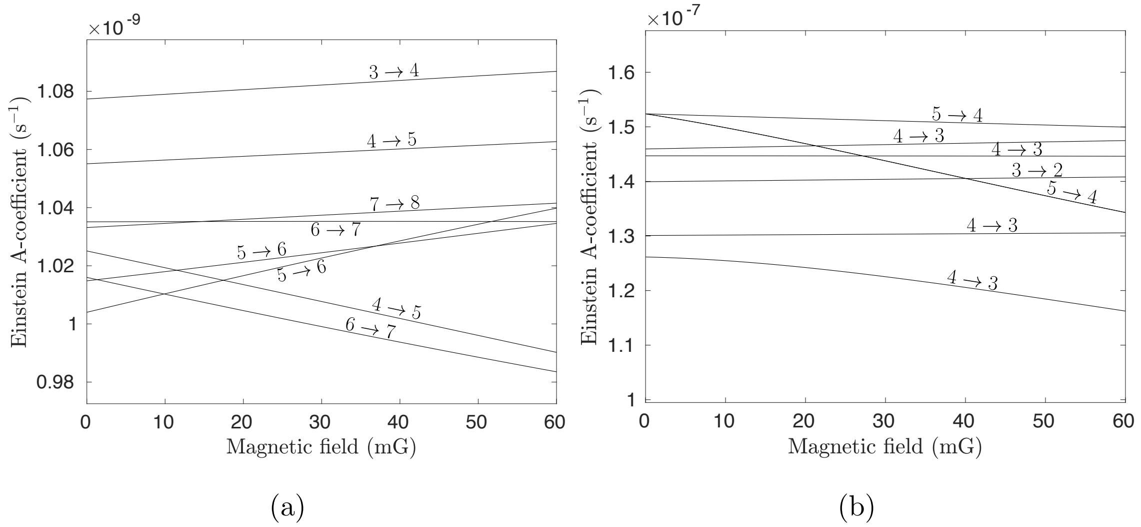


Supplementary Figure 2: Magnetic field dependence of the Einstein A-coefficients of the strongest hyperfine transitions within the 6.7 GHz ($5_{15}$ $A_2 \rightarrow 6_{06}$ $A_1$) (a) and 36 GHz ($4_{-1}$ $E \rightarrow 3_0$ $E$) (b) methanol maser lines

## ROTATIONAL AND TORSIONAL ZEEMAN EFFECTS

The method section of the paper describes the formalism that we used to compute the Zeeman effects in methanol. Here, we present a rigorous derivation of this formalism.

Molecules consist of charged particles, nuclei and electrons, and their rotation produces a magnetic dipole moment. For molecules with internal rotation, such as methanol, an additional magnetic dipole moment originates from their torsional motion. These magnetic moments, interacting with the nuclear spins, are involved in the molecules' hyperfine structure. The derivation of the appropriate hyperfine Hamiltonian was described by Lankhaar *et al.*[1]. Here, we derive the corresponding Zeeman Hamiltonian for the interaction of the rotational and torsional magnetic moments with external magnetic fields. We refer to Appendix A of Ref. [1] for most of the theoretical background.

As usual for molecules with internal rotation, we distinguish two parts of the molecule that are internally rigid. The "frame" part consists of those atoms that remain fixed in the molecule-fixed (MF) principal axis frame, in the case of methanol the OH fragment. The origin of the MF frame is the center of mass of the $CH_3OH$ molecule and its orientation with respect to a space-fixed (SF) frame is defined by three Euler angles $(\chi, \theta, \phi)$. The "top" part is fixed with respect to a frame TF that rotates with respect to the MF frame about

a single (fixed) axis $\boldsymbol{\lambda}$ over an angle $\gamma$. This "top" is considered to be a symmetric rotor, such as the $CH_3$ group in methanol.

The magnetic moment of methanol, $\boldsymbol{m}$, is determined by all the moving charged particles[2]

$$\boldsymbol{m} = \frac{1}{2}\sum_i Q_i(\boldsymbol{r}_i \times \boldsymbol{v}_i), \tag{2}$$

where $\boldsymbol{r}_i$, $Q_i$ and $\boldsymbol{v}_i$ are the position, charge, and velocity of particle $i$. Electrons have $Q_i = -e$ and nuclei have charge $Z_i e$ with $Z_i$ given by their atomic number. The energy of this magnetic moment in a (homogeneous) external magnetic field $\boldsymbol{B}$ is

$$H = -\boldsymbol{B}\cdot\boldsymbol{m} = -\sum_i \frac{Q_i}{2}\boldsymbol{B}\cdot(\boldsymbol{r}_i \times \boldsymbol{v}_i), \tag{3}$$

In this summation we can distinguish between particles in the "frame" and particles in the "top", of which the positions are fixed with respect to the MF and TF frame, respectively. Their positions with respect to the SF frame are given by equation (A1) of Ref. [1], and in equation (A3) of Ref. [1] their velocities are expressed in terms of the angular velocity $\boldsymbol{\omega}$ of the whole molecule and the velocity $\dot{\gamma}$ of rotation of the "top" about the axis $\boldsymbol{\lambda}$ relative to the "frame". Substitution of these expressions into Supplementary equation (3) yields

$$H^{\text{frame}} = -\boldsymbol{B}\cdot\boldsymbol{V}^{\text{frame}}\boldsymbol{\omega}, \tag{4}$$

for particles in the "frame", with

$$\boldsymbol{V}^{\text{frame}} = \sum_i^{\text{frame}} \frac{Q_i}{2}[(\boldsymbol{r}_i^{\text{MF}}\cdot\boldsymbol{r}_i^{\text{MF}})\mathbf{1} - \boldsymbol{r}_i^{\text{MF}}\otimes\boldsymbol{r}_i^{\text{MF}}] \tag{5}$$

For particles in the "top" we obtain

$$H^{\text{top}} = -\boldsymbol{B}\cdot\boldsymbol{V}^{\text{top}}\boldsymbol{\omega}' - \boldsymbol{B}\cdot\boldsymbol{v}\dot{\gamma}, \tag{6}$$

with

$$\boldsymbol{V}^{\text{top}} = \sum_i^{\text{top}} \frac{Q_i}{2}[(\boldsymbol{r}_i^{\text{TF}}\cdot\boldsymbol{r}_i^{\text{TF}})\mathbf{1} - \boldsymbol{r}_i^{\text{TF}}\otimes\boldsymbol{r}_i^{\text{TF}}], \tag{7}$$

and

$$\boldsymbol{v} = \sum_i^{\text{top}} \frac{Q_i}{2}[(\boldsymbol{r}_i^{\text{TF}}\cdot\boldsymbol{r}_i^{\text{TF}})\mathbf{1} - \boldsymbol{r}_i^{\text{TF}}\otimes\boldsymbol{r}_i^{\text{TF}}]\boldsymbol{\lambda}. \tag{8}$$

The angular velocity $\boldsymbol{\omega}'$ with respect to the TF frame is related to $\boldsymbol{\omega}$ defined in the MF frame as $\boldsymbol{\omega}' = \boldsymbol{R}(\boldsymbol{\lambda},\gamma)\boldsymbol{\omega}$, where $\boldsymbol{R}(\boldsymbol{\lambda},\gamma)$ represents the rotation over $\gamma$ about axis $\boldsymbol{\lambda}$. All

tensor and vector components in Supplementary equations (6), (7), and (8) are defined in the TF frame, while Supplementary equations (4) and (5) are written in the MF frame. We prefer to write all equations in the MF frame, i.e., the principal axes frame of the whole molecule. This can be achieved by transformation to the $\gamma$ dependent coupling tensor $\boldsymbol{V}^{\rm top}(\gamma) = \boldsymbol{R}(\boldsymbol{\lambda},\gamma)^{-1}\boldsymbol{V}^{\rm top}\boldsymbol{R}(\boldsymbol{\lambda},\gamma)$ and coupling vector $\boldsymbol{v}(\gamma) = \boldsymbol{R}(\boldsymbol{\lambda},\gamma)^{-1}\boldsymbol{v}$. Supplementary equation (6) then becomes

$$H^{\rm top} = -\boldsymbol{B}\cdot\boldsymbol{V}^{\rm top}(\gamma)\boldsymbol{\omega} - \boldsymbol{B}\cdot\boldsymbol{v}(\gamma)\dot{\gamma}, \tag{9}$$

in which also the components of $\boldsymbol{B}$ and $\boldsymbol{\omega}$ are given in the MF frame. Since all tensors and vectors are now given in the MF frame, we may add Supplementary equations (4) and (9) to obtain

$$H = -\boldsymbol{B}\cdot\boldsymbol{V}(\gamma)\boldsymbol{\omega} - \boldsymbol{B}\cdot\boldsymbol{v}(\gamma)\dot{\gamma}, \tag{10}$$

with

$$\begin{aligned}\boldsymbol{V}(\gamma) &= \boldsymbol{V}^{\rm frame} + \boldsymbol{V}^{\rm top}(\gamma)\\ &= \sum_i \frac{Q_i}{2}\left[(\boldsymbol{r}_i^{\rm MF}\cdot\boldsymbol{r}_i^{\rm MF})\mathbf{1} - \boldsymbol{r}_i^{\rm MF}\otimes\boldsymbol{r}_i^{\rm MF}\right],\end{aligned} \tag{11}$$

where the sum over particles $i$ now runs over all electrons and nuclei in the whole molecule. We note that the positions $\boldsymbol{r}_i^{\rm MF}$ of particles in the top depend on the internal rotation angle $\gamma$.

Next we replace the angular velocities $\boldsymbol{\omega}$ and $\dot{\gamma}$ in Supplementary equation (10) by their conjugate angular momenta $\boldsymbol{J}$ and $p_\gamma$, with the use of equation (A7) from Ref. [1]. The quantum mechanical equivalent is then obtained by replacing the angular momenta $\boldsymbol{J}$ and $p_\gamma$ by the corresponding operators $\hat{\boldsymbol{J}}$ and $(\hbar/i)\partial/\partial\gamma$. This yields $H \to \hat{H} = \hat{H}_{\rm BR} + \hat{H}_{\rm BT}$, with the rotational and torsional Zeeman Hamiltonians $\hat{H}_{\rm BR}$ and $\hat{H}_{\rm BT}$ given in equations (1) and (2) in the Methods section of the paper. The coupling tensors are defined as

$$\boldsymbol{g}(\gamma) = \frac{\hbar}{\mu_N}\boldsymbol{V}(\gamma)\boldsymbol{I}^{-1} \tag{12}$$

and

$$\boldsymbol{b}(\gamma) = \frac{\hbar}{\mu_N}\boldsymbol{v}(\gamma)I_\gamma^{-1}, \tag{13}$$

where $I_\gamma$ is the moment of inertia of the "top" about the rotation axis $\boldsymbol{\lambda}$ and $\boldsymbol{I}$ the inertia tensor of the whole molecule, which is diagonal in the principal axes frame MF.

Finally we note that the coupling tensors given in Supplementary equations (8) and (11) depend on the coordinates of both nuclei and electrons. The contributions that contain the nuclear coordinates can be directly calculated, since the positions of the nuclei are fixed with respect to the MF frame (for the nuclei in the "frame") or depend only on the torsion angle $\gamma$ (for the nuclei in the "top"). For the rotational Zeeman coupling tensor $\boldsymbol{g}$ it was shown that the electronic contributions can be obtained by second order perturbation theory [3] with matrix elements over the molecule's ground state and excited electronic wave functions. Calculation of this rotational Zeeman tensor has been implemented in the electronic structure program package CFOUR[4], and it can thus be computed as a function of $\gamma$. No such implementation yet exists, however, for the torsional Zeeman coupling vector $\boldsymbol{b}$. A procedure to estimate this b-vector with the use of experimental data[5] is described in the paper.

Supplementary Table 1: Coefficients $a_n$ in the Fourier expansion describing the torsional angle $\gamma$ dependence of the rotational g-tensor calculated *ab initio*. The ($\gamma$-independent) components of the torsion-magnetic field coupling vector $\boldsymbol{b}(\gamma)$ have been estimated from experimental data, see text. The components of $\boldsymbol{g}(\gamma)$ and $\boldsymbol{b}(\gamma)$ are defined with respect to the principal axes $\boldsymbol{a}$, $\boldsymbol{b}$, and $\boldsymbol{c}$ of methanol. Terms in the Fourier series are $\cos n\gamma$ or $\sin n\gamma$, depending on whether a component is symmetric (+) or antisymmetric (−) with respect to a sign change of $\gamma$.

| | Symmetry | $a_0$ | $a_3$ | $a_6$ |
|---|---|---|---|---|
| $g_{aa}$ | + | 0.325 | 0.0165 | $4.86 \times 10^{-5}$ |
| $g_{bb}$ | + | −0.056 | −0.0014 | $1.04 \times 10^{-5}$ |
| $g_{cc}$ | + | −0.033 | $-1.25 \times 10^{-3}$ | $7.0 \times 10^{-6}$ |
| $g_{ab}$ | + | 0.139 | −0.019 | $2.04 \times 10^{-5}$ |
| $g_{ba}$ | + | 0.027 | $-3.65 \times 10^{-3}$ | $4.0 \times 10^{-6}$ |
| $g_{ac}$ | − | 0 | 0.014 | $3.15 \times 10^{-5}$ |
| $g_{ca}$ | − | 0 | $2.69 \times 10^{-3}$ | $5.8 \times 10^{-6}$ |
| $g_{bc}$ | − | 0 | $2.97 \times 10^{-4}$ | $-7.0 \times 10^{-6}$ |
| $g_{cb}$ | − | 0 | $2.87 \times 10^{-4}$ | $-6.8 \times 10^{-6}$ |
| $b_a$ | + | 0.346 | 0 | 0 |
| $b_b$ | + | 0.019 | 0 | 0 |
| $b_c$ | − | 0 | 0 | 0 |

## EFFECTIVE ZEEMAN HAMILTONIAN

It is mentioned in the paper that in order to obtain the magnetic field dependent spectrum of methanol we needed to compute the matrix elements of the Zeeman Hamiltonian. The evaluation of these matrix elements can be considerably simplified by the use of an *effective* Zeeman Hamiltonian similar to the effective hyperfine Hamiltonian in Ref. [1]. Since in methanol the energy gaps between torsion-rotation states are typically larger than the hyperfine and Zeeman splittings by several orders of magnitude, we may restrict the basis to a single value of the torsional and rotational quantum numbers $v_\tau$ and $J$. In analogy with the expressions for the hyperfine interactions in Section III.B.3 of Ref. [1] and basing

ourselves on the literature[6–9], we can then derive an effective Zeeman Hamiltonian that gives exactly the same matrix elements as the Zeeman Hamiltonian in equation (5) of the paper. This effective Zeeman Hamiltonian reads

$$\hat{H}_{\text{Zeeman}} = -\frac{\mu_N}{\hbar} g_p \sum_K \boldsymbol{B} \cdot \hat{\boldsymbol{I}}_K - \frac{\mu_N}{\hbar} \left(\hat{g}_{\text{BR}} + \hat{g}_{\text{BT}}\right) (\boldsymbol{B} \cdot \hat{\boldsymbol{J}}). \tag{14}$$

The advantage of this factorization is that the scalar product operators $\hat{\boldsymbol{B}} \cdot \hat{\boldsymbol{I}}_K$ and $\hat{\boldsymbol{B}} \cdot \hat{\boldsymbol{J}}$ are invariant under rotation, which we used to express them in terms of the space-fixed (SF) components of the operators. Matrix elements over the SF basis $|\{(I_{123}, I_4)I, J\}FM_F\rangle$ are thus more easily evaluated. The operators

$$\hat{g}_{\text{BR}} = \frac{1}{2J(J+1)} \hat{\boldsymbol{J}} \cdot \boldsymbol{g}(\gamma) \hat{\boldsymbol{J}} + \text{hermitian conjugate}$$

$$\hat{g}_{\text{BT}} = \frac{f}{2J(J+1)} \hat{\boldsymbol{J}} \cdot \boldsymbol{b}'(\gamma) \left(\hat{p}_\gamma - \boldsymbol{\rho} \cdot \hat{\boldsymbol{J}}\right) + \text{hermitian conjugate}, \tag{15}$$

contain the body-fixed components of $\hat{\boldsymbol{J}}$ with respect to the MF frame[1], and also the tensors $\boldsymbol{g}(\gamma)$ and $\boldsymbol{b}'(\gamma)$ are given with respect to this frame. Matrix elements of the operators $\hat{g}_{\text{BR}}$ and $\hat{g}_{\text{BT}}$ over the torsion-rotation eigenfunctions are simply scalar values: the g-factors belonging to a certain torsion-rotation level.

## CHARACTERISTICS OF METHANOL'S MASER TRANSITIONS

In the following Supplementary Tables 2-18 below we summarize the relevant parameters for the individual hyperfine transitions in all known methanol maser lines. For the strongest hyperfine components with $\Delta F = F_{\rm down} - F_{\rm up} = \Delta J$, we list the following parameters: the hyperfine frequency shift $\Delta E$ relative to the frequency of the corresponding torsion-rotation transition, the Landé g-factors $g_l$ at 10 mG which are dimensionless, and the Zeeman-splitting coefficients, $\alpha_Z = \mu_N g_l$ in Hz mG$^{-1}$ and in m s$^{-1}$G$^{-1}$ ($c\alpha_Z/f$). The constants $\mu_N$, $c$, and $f$ are the nuclear magneton, the speed of light (in m/s), and the frequency of the transition (in Hz). In the last column we report the Einstein A-coefficients of the hyperfine transitions in zero magnetic field.

Supplementary Table 2: 107 GHz ($3_{13}$ $A_2 \rightarrow 4_{04}$ $A_1$)

| $F_{\rm up}$ | $F_{\rm down}$ | $\Delta E$ (kHz) | $g_l$ | $\alpha_Z$(Hz mG$^{-1}$) | $\alpha_Z$(m s$^{-1}$G$^{-1}$) | $A$ ($10^{-8}$ s$^{-1}$) |
|---|---|---|---|---|---|---|
| 5 | 6 | 3.059 | 0.844 | 0.644 | 1.803 | 380.097 |
| 4 | 5 | −6.620 | 0.727 | 0.554 | 1.553 | 351.726 |
| 4 | 5 | 5.151 | 0.218 | 0.166 | 0.465 | 327.388 |
| 3 | 4 | −2.873 | −0.297 | −0.226 | −0.633 | 357.762 |
| 3 | 4 | 3.639 | 0.125 | 0.095 | 0.267 | 350.923 |
| 2 | 3 | −0.999 | −0.903 | −0.688 | −1.929 | 391.419 |
| 2 | 3 | −2.968 | −1.140 | −0.869 | −2.434 | 361.512 |
| 1 | 2 | −6.894 | −2.893 | −2.205 | −6.177 | 413.509 |

Supplementary Table 3: 6.7 GHz ($5_{15}$ $A_2 \rightarrow 6_{06}$ $A_1$)

| $F_{\rm up}$ | $F_{\rm down}$ | $\Delta E$ (kHz) | $g_l$ | $\alpha_Z$(Hz mG$^{-1}$) | $\alpha_Z$(m s$^{-1}$G$^{-1}$) | $A$ ($10^{-8}$ s$^{-1}$) |
|---|---|---|---|---|---|---|
| 7 | 8 | 2.500 | 0.619 | 0.472 | 21.176 | 0.103 |
| 6 | 7 | −4.397 | 0.342 | 0.261 | 11.716 | 0.104 |
| 6 | 7 | 3.541 | 0.294 | 0.224 | 10.067 | 0.102 |
| 5 | 6 | −2.889 | −0.167 | −0.127 | −5.712 | 0.101 |
| 5 | 6 | 3.015 | 0.002 | 0.002 | 0.070 | 0.100 |
| 4 | 5 | 1.240 | −0.612 | −0.467 | −20.963 | 0.106 |
| 4 | 5 | −2.835 | −0.677 | −0.516 | −23.187 | 0.103 |
| 3 | 4 | −4.417 | −1.489 | −1.135 | −50.955 | 0.108 |

Supplementary Table 4: 44 GHz ($7_{07}$ $A_2 \rightarrow 6_{16}$ $A_1$ )

| $F_{\rm up}$ | $F_{\rm down}$ | $\Delta E$ (kHz) | $g_l$ | $\alpha_Z$(Hz mG$^{-1}$) | $\alpha_Z$(m s$^{-1}$G$^{-1}$) | $A$ ($10^{-8}$ s$^{-1}$) |
|---|---|---|---|---|---|---|
| 9 | 8 | −2.444 | 0.542 | 0.413 | 2.811 | 27.449 |
| 8 | 7 | 3.934 | 0.267 | 0.203 | 1.383 | 27.116 |
| 8 | 7 | −3.216 | 0.272 | 0.207 | 1.409 | 26.796 |
| 7 | 6 | 2.897 | −0.142 | −0.108 | −0.736 | 26.285 |
| 7 | 6 | −2.897 | −0.022 | −0.016 | −0.112 | 26.078 |
| 6 | 5 | −1.684 | −0.529 | −0.403 | −2.745 | 26.407 |
| 6 | 5 | 2.863 | −0.572 | −0.436 | −2.966 | 25.874 |
| 5 | 4 | 3.998 | −1.207 | −0.920 | −6.260 | 25.913 |

Supplementary Table 5: 95 GHz ($8_{08}$ $A_1 \rightarrow 7_{17}$ $A_2$)

| $F_{\text{up}}$ | $F_{\text{down}}$ | $\Delta E$ (kHz) | $g_l$ | $\alpha_Z$(Hz mG$^{-1}$) | $\alpha_Z$(m s$^{-1}$G$^{-1}$) | $A$ ($10^{-8}$ s$^{-1}$) |
|---|---|---|---|---|---|---|
| 10 | 9 | −2.464 | 0.480 | 0.366 | 1.153 | 286.937 |
| 9 | 8 | 3.666 | 0.207 | 0.158 | 0.497 | 283.586 |
| 9 | 8 | −3.047 | 0.254 | 0.194 | 0.611 | 281.444 |
| 8 | 7 | 2.941 | −0.126 | −0.096 | −0.304 | 277.656 |
| 8 | 7 | −2.864 | −0.037 | −0.028 | −0.088 | 276.014 |
| 7 | 6 | −2.002 | −0.468 | −0.357 | −1.125 | 278.775 |
| 7 | 6 | 2.929 | −0.499 | −0.380 | −1.197 | 274.546 |
| 6 | 5 | 3.788 | −1.019 | −0.777 | −2.448 | 275.165 |

Supplementary Table 6: 104 GHz ($11_{-1}$ $E \rightarrow 10_{-2}$ $E$)

| $F_{\text{up}}$ | $F_{\text{down}}$ | $\Delta E$ (kHz) | $g_l$ | $\alpha_Z$(Hz mG$^{-1}$) | $\alpha_Z$(m s$^{-1}$G$^{-1}$) | $A$ ($10^{-8}$ s$^{-1}$) |
|---|---|---|---|---|---|---|
| 12 | 11 | −1.879 | 0.154 | 0.117 | 0.338 | 134.346 |
| 11 | 10 | 3.181 | −0.087 | −0.066 | −0.190 | 133.740 |
| 11 | 10 | −1.246 | −0.073 | −0.055 | −0.159 | 133.680 |
| 10 | 9 | 1.859 | −0.360 | −0.275 | −0.790 | 133.128 |
| 12 | 11 | −3.047 | 0.158 | 0.120 | 0.345 | 134.346 |
| 11 | 10 | 1.915 | −0.086 | −0.065 | −0.188 | 133.761 |
| 11 | 10 | −1.246 | −0.077 | −0.059 | −0.169 | 133.679 |
| 10 | 9 | 3.244 | −0.361 | −0.275 | −0.792 | 133.128 |

Supplementary Table 7: 12.2 GHz ($2_0$ $E \rightarrow 3_{-1}$ $E$)

| $F_{\mathrm{up}}$ | $F_{\mathrm{down}}$ | $\Delta E$ (kHz) | $g_l$ | $\alpha_Z$(Hz mG$^{-1}$) | $\alpha_Z$(m s$^{-1}$G$^{-1}$) | $A$ ($10^{-8}$ s$^{-1}$) |
|---|---|---|---|---|---|---|
| 3 | 4 | −4.965 | 0.714 | 0.544 | 13.401 | 0.737 |
| 2 | 3 | −4.802 | 0.144 | 0.110 | 2.706 | 0.752 |
| 2 | 3 | −1.475 | −0.117 | −0.089 | −2.193 | 0.732 |
| 1 | 2 | 7.978 | −1.433 | −1.093 | −26.897 | 0.803 |
| 3 | 4 | −6.106 | 0.614 | 0.468 | 11.516 | 0.737 |
| 2 | 3 | 5.847 | 0.385 | 0.294 | 7.230 | 0.610 |
| 2 | 3 | −1.475 | −0.218 | −0.166 | −4.092 | 0.571 |
| 1 | 2 | 3.263 | −1.397 | −1.065 | −26.221 | 0.803 |

Supplementary Table 8: 24.934 GHz ($2_2$ $E \rightarrow 2_1$ $E$)

| $F_{\mathrm{up}}$ | $F_{\mathrm{down}}$ | $\Delta E$ (kHz) | $g_l$ | $\alpha_Z$(Hz mG$^{-1}$) | $\alpha_Z$(m s$^{-1}$G$^{-1}$) | $A$ ($10^{-8}$ s$^{-1}$) |
|---|---|---|---|---|---|---|
| 3 | 3 | 16.247 | 2.072 | 1.579 | 18.987 | 3.553 |
| 2 | 2 | 9.941 | 0.261 | 0.199 | 2.390 | 3.479 |
| 2 | 2 | −23.440 | 0.549 | 0.418 | 5.029 | 3.209 |
| 1 | 1 | −18.416 | −2.530 | −1.929 | −23.188 | 2.998 |
| 3 | 3 | 14.961 | 1.914 | 1.459 | 17.539 | 3.553 |
| 2 | 2 | 11.751 | 0.443 | 0.337 | 4.057 | 3.498 |
| 2 | 2 | −23.440 | 0.576 | 0.439 | 5.281 | 3.205 |
| 1 | 1 | −15.427 | −2.556 | −1.948 | −23.421 | 2.998 |

Supplementary Table 9: 24.929 GHz ($3_2\ E \rightarrow 3_1\ E$)

| $F_{\rm up}$ | $F_{\rm down}$ | $\Delta E$ (kHz) | $g_l$ | $\alpha_Z$(Hz mG$^{-1}$) | $\alpha_Z$(m s$^{-1}$G$^{-1}$) | $A$ ($10^{-8}$ s$^{-1}$) |
|---|---|---|---|---|---|---|
| 4 | 4 | 8.336 | 1.410 | 1.075 | 12.926 | 4.699 |
| 3 | 3 | 8.365 | 0.226 | 0.172 | 2.067 | 4.641 |
| 3 | 3 | −10.893 | 0.293 | 0.224 | 2.690 | 4.543 |
| 2 | 2 | −7.813 | −1.844 | −1.405 | −16.898 | 4.456 |
| 4 | 4 | 10.388 | 1.460 | 1.113 | 13.377 | 4.699 |
| 3 | 3 | 5.704 | 0.172 | 0.131 | 1.576 | 4.630 |
| 3 | 3 | −10.893 | 0.280 | 0.213 | 2.565 | 4.541 |
| 2 | 2 | −11.434 | −1.830 | −1.395 | −16.776 | 4.456 |

Supplementary Table 10: 36 GHz ($4_{-1}\ E \rightarrow 3_0\ E$)

| $F_{\rm up}$ | $F_{\rm down}$ | $\Delta E$ (kHz) | $g_l$ | $\alpha_Z$(Hz mG$^{-1}$) | $\alpha_Z$(m s$^{-1}$G$^{-1}$) | $A$ ($10^{-8}$ s$^{-1}$) |
|---|---|---|---|---|---|---|
| 5 | 4 | 5.402 | 0.638 | 0.486 | 4.032 | 15.238 |
| 4 | 3 | −4.791 | 0.228 | 0.174 | 1.442 | 13.009 |
| 4 | 3 | −3.395 | −0.359 | −0.274 | −2.270 | 12.615 |
| 3 | 2 | −3.032 | −0.944 | −0.720 | −5.965 | 13.994 |
| 5 | 4 | 4.042 | 0.556 | 0.424 | 3.514 | 15.238 |
| 4 | 3 | 4.303 | 0.073 | 0.056 | 0.461 | 14.595 |
| 4 | 3 | −3.395 | −0.098 | −0.075 | −0.619 | 14.469 |
| 3 | 2 | −6.802 | −0.924 | −0.704 | −5.836 | 13.995 |

Supplementary Table 11: 24.933 GHz ($4_2$ $E \to 4_1$ $E$)

| $F_{\rm up}$ | $F_{\rm down}$ | $\Delta E$ (kHz) | $g_l$ | $\alpha_Z$(Hz mG$^{-1}$) | $\alpha_Z$(m s$^{-1}$G$^{-1}$) | $A$ ($10^{-8}$ s$^{-1}$) |
|---|---|---|---|---|---|---|
| 5 | 5 | 6.560 | 1.157 | 0.882 | 10.603 | 5.266 |
| 4 | 4 | 2.449 | 0.077 | 0.059 | 0.706 | 5.216 |
| 4 | 4 | −8.496 | 0.139 | 0.106 | 1.269 | 5.189 |
| 3 | 3 | −6.955 | −1.397 | −1.065 | −12.797 | 5.142 |
| 5 | 5 | 3.679 | 1.118 | 0.852 | 10.245 | 5.266 |
| 4 | 4 | 5.997 | 0.120 | 0.091 | 1.098 | 5.220 |
| 4 | 4 | −8.496 | 0.150 | 0.114 | 1.371 | 5.190 |
| 3 | 3 | −2.567 | −1.409 | −1.074 | −12.908 | 5.142 |

Supplementary Table 12: 85 GHz ($5_{-1}$ $E \to 4_0$ $E$)

| $F_{\rm up}$ | $F_{\rm down}$ | $\Delta E$ (kHz) | $g_l$ | $\alpha_Z$(Hz mG$^{-1}$) | $\alpha_Z$(m s$^{-1}$G$^{-1}$) | $A$ ($10^{-8}$ s$^{-1}$) |
|---|---|---|---|---|---|---|
| 6 | 5 | 3.452 | 0.457 | 0.348 | 1.235 | 87.938 |
| 5 | 4 | 3.930 | 0.043 | 0.033 | 0.117 | 85.226 |
| 5 | 4 | 1.095 | −0.081 | −0.062 | −0.220 | 84.935 |
| 4 | 3 | −6.089 | −0.703 | −0.536 | −1.902 | 83.595 |
| 6 | 5 | 4.919 | 0.514 | 0.392 | 1.389 | 87.937 |
| 5 | 4 | −4.236 | 0.139 | 0.106 | 0.376 | 79.686 |
| 5 | 4 | 1.095 | −0.242 | −0.185 | −0.655 | 78.343 |
| 4 | 3 | −2.630 | −0.717 | −0.547 | −1.939 | 83.595 |

Supplementary Table 13: 24.959 GHz ($5_2$ $E \to 5_1$ $E$)

| $F_{\mathrm{up}}$ | $F_{\mathrm{down}}$ | $\Delta E$ (kHz) | $g_l$ | $\alpha_Z$(Hz mG$^{-1}$) | $\alpha_Z$(m s$^{-1}$G$^{-1}$) | $A$ ($10^{-8}$ s$^{-1}$) |
|---|---|---|---|---|---|---|
| 6 | 6 | −0.026 | 0.929 | 0.708 | 8.495 | 5.570 |
| 5 | 5 | 4.223 | 0.059 | 0.045 | 0.541 | 5.538 |
| 5 | 5 | −1.070 | 0.082 | 0.062 | 0.750 | 5.533 |
| 4 | 4 | 1.462 | −1.145 | −0.873 | −10.473 | 5.500 |
| 6 | 6 | 3.754 | 0.961 | 0.732 | 8.788 | 5.570 |
| 5 | 5 | −0.271 | 0.024 | 0.018 | 0.222 | 5.537 |
| 5 | 5 | −1.070 | 0.071 | 0.054 | 0.652 | 5.532 |
| 4 | 4 | −3.784 | −1.133 | −0.864 | −10.364 | 5.500 |

Supplementary Table 14: 25.018 GHz ($6_2$ $E \to 6_1$ $E$)

| $F_{\mathrm{up}}$ | $F_{\mathrm{down}}$ | $\Delta E$ (kHz) | $g_l$ | $\alpha_Z$(Hz mG$^{-1}$) | $\alpha_Z$(m s$^{-1}$G$^{-1}$) | $A$ ($10^{-8}$ s$^{-1}$) |
|---|---|---|---|---|---|---|
| 7 | 7 | 1.562 | 0.820 | 0.625 | 7.485 | 5.887 |
| 6 | 6 | 2.035 | 0.034 | 0.026 | 0.308 | 5.869 |
| 6 | 6 | 2.840 | −0.006 | −0.005 | −0.057 | 5.865 |
| 5 | 5 | −1.375 | −0.955 | −0.728 | −8.712 | 5.843 |
| 7 | 7 | −3.193 | 0.796 | 0.607 | 7.261 | 5.887 |
| 6 | 6 | −3.232 | 0.045 | 0.034 | 0.407 | 5.869 |
| 6 | 6 | 2.840 | 0.020 | 0.015 | 0.184 | 5.865 |
| 5 | 5 | 4.817 | −0.967 | −0.737 | −8.821 | 5.843 |

Supplementary Table 15: 25.125 GHz ($7_2$ $E \rightarrow 7_1$ $E$)

| $F_{\rm up}$ | $F_{\rm down}$ | $\Delta E$ (kHz) | $g_l$ | $\alpha_Z$(Hz mG$^{-1}$) | $\alpha_Z$(m s$^{-1}$G$^{-1}$) | $A$ ($10^{-8}$ s$^{-1}$) |
|---|---|---|---|---|---|---|
| 8 | 8 | −6.018 | 0.698 | 0.532 | 6.343 | 6.085 |
| 7 | 7 | −1.648 | 0.022 | 0.017 | 0.200 | 6.075 |
| 7 | 7 | −4.870 | −0.007 | −0.005 | −0.065 | 6.068 |
| 6 | 6 | 7.756 | −0.839 | −0.639 | −7.618 | 6.055 |
| 8 | 8 | −0.203 | 0.715 | 0.545 | 6.489 | 6.085 |
| 7 | 7 | 4.646 | 0.011 | 0.008 | 0.096 | 6.075 |
| 7 | 7 | −4.870 | −0.024 | −0.019 | −0.220 | 6.068 |
| 6 | 6 | 0.524 | −0.827 | −0.630 | −7.507 | 6.055 |

Supplementary Table 16: 25.294 GHz ($8_2$ $E \rightarrow 8_1$ $E$)

| $F_{\rm up}$ | $F_{\rm down}$ | $\Delta E$ (kHz) | $g_l$ | $\alpha_Z$(Hz mG$^{-1}$) | $\alpha_Z$(m s$^{-1}$G$^{-1}$) | $A$ ($10^{-8}$ s$^{-1}$) |
|---|---|---|---|---|---|---|
| 9 | 9 | −1.631 | 0.632 | 0.482 | 5.695 | 6.455 |
| 8 | 8 | 6.946 | −0.005 | −0.004 | −0.044 | 6.448 |
| 8 | 8 | 0.893 | −0.035 | −0.027 | −0.319 | 6.438 |
| 7 | 7 | 2.029 | −0.730 | −0.556 | −6.580 | 6.433 |
| 9 | 9 | −8.594 | 0.625 | 0.477 | 5.637 | 6.455 |
| 8 | 8 | −0.466 | 0.007 | 0.006 | 0.065 | 6.448 |
| 8 | 8 | 0.893 | −0.029 | −0.022 | −0.259 | 6.440 |
| 7 | 7 | 10.402 | −0.743 | −0.566 | −6.694 | 6.433 |

Supplementary Table 17: 9.91 GHz ($9_{-1}$ $E \rightarrow 8_{-2}$ $E$)

| $F_{\mathrm{up}}$ | $F_{\mathrm{down}}$ | $\Delta E$ (kHz) | $g_l$ | $\alpha_Z$(Hz mG$^{-1}$) | $\alpha_Z$(m s$^{-1}$G$^{-1}$) | $A$ ($10^{-8}$ s$^{-1}$) |
|---|---|---|---|---|---|---|
| 10 | 9 | −3.418 | 0.187 | 0.143 | 4.319 | 0.113 |
| 9 | 8 | 4.343 | −0.105 | −0.080 | −2.416 | 0.112 |
| 9 | 8 | −2.360 | −0.084 | −0.064 | −1.933 | 0.112 |
| 8 | 7 | 3.809 | −0.445 | −0.339 | −10.261 | 0.112 |
| 10 | 9 | −4.433 | 0.193 | 0.147 | 4.452 | 0.113 |
| 9 | 8 | 3.679 | −0.109 | −0.083 | −2.514 | 0.112 |
| 9 | 8 | −2.360 | −0.086 | −0.065 | −1.981 | 0.112 |
| 8 | 7 | 4.509 | −0.445 | −0.340 | −10.271 | 0.112 |

Supplementary Table 18: 25.541 GHz ($9_2$ $E \rightarrow 9_1$ $E$)

| $F_{\mathrm{up}}$ | $F_{\mathrm{down}}$ | $\Delta E$ (kHz) | $g_l$ | $\alpha_Z$(Hz mG$^{-1}$) | $\alpha_Z$(m s$^{-1}$G$^{-1}$) | $A$ ($10^{-8}$ s$^{-1}$) |
|---|---|---|---|---|---|---|
| 10 | 10 | −10.965 | 0.571 | 0.435 | 5.091 | 6.705 |
| 9 | 9 | 0.398 | −0.003 | −0.002 | −0.025 | 6.699 |
| 9 | 9 | −8.830 | −0.049 | −0.037 | −0.434 | 6.691 |
| 8 | 8 | 12.815 | −0.667 | −0.509 | −5.955 | 6.689 |
| 10 | 10 | −2.762 | 0.565 | 0.431 | 5.042 | 6.705 |
| 9 | 9 | 9.022 | −0.016 | −0.012 | −0.139 | 6.695 |
| 9 | 9 | −8.830 | −0.042 | −0.032 | −0.378 | 6.685 |
| 8 | 8 | 3.197 | −0.654 | −0.499 | −5.838 | 6.689 |

[1] Lankhaar, B., Groenenboom, G. C. & van der Avoird, A. Hyperfine interactions and internal rotation in methanol. *J. Chem. Phys.* **145**, 244301 (2016).

[2] Jackson, J. D. *Classical electrodynamics* (Wiley, New York, 1998), third edn.

[3] Flygare, W. H. Spin-rotation interaction and magnetic shielding in molecules. *J. Chem. Phys.* **41**, 793–800 (1964).

[4] Stanton, J., Gauss, J., M.E., H. & Szalay, P. CFOUR, Coupled-Cluster techniques for Computational Chemistry. Http://www.cfour.de.

[5] Engelbrecht, L. & Sutter, D. The rotational Zeeman effect of molecules with low barrier internal rotation. II. Derivation of the effective rotorsional hamiltonian. *Z. Naturforsch. A* **33**, 1525–1545 (1978).

[6] Hougen, J. T. Reinterpretation of molecular beam hyperfine data for $^{14}NH_3$ and $^{15}NH_3$. *J. Chem. Phys.* **57**, 4207–4217 (1972).

[7] Hougen, J. T., Meerts, W. L. & Ozier, I. The use of extended permutation-inversion groups in constructing hyperfine hamiltonians for symmetric-top internal rotor molecules like $H_3CSiH_3$. *J. Mol. Spectrosc.* **146**, 8–48 (1991).

[8] Coudert, L. H., Caminati, W., Schnell, M. & Grabow, J.-U. Hyperfine coupling and large amplitude motions interaction in the water dimer. *J. Mol. Spectrosc.* **242**, 118–128 (2007).

[9] Tudorie, M., Coudert, L. H., Huet, T. R., Jegouso, D. & Sedes, G. Magnetic hyperfine coupling of a methyl group undergoing internal rotation: A case study of methyl formate. *J. Chem. Phys.* **134**, 074314 (2011).
